# Supplementary material for: Group Diffusion: Enhancing Image Generation by Unlocking Cross-Sample Collaboration
Source: arXiv:2512.10954 source file (2025-12-11)

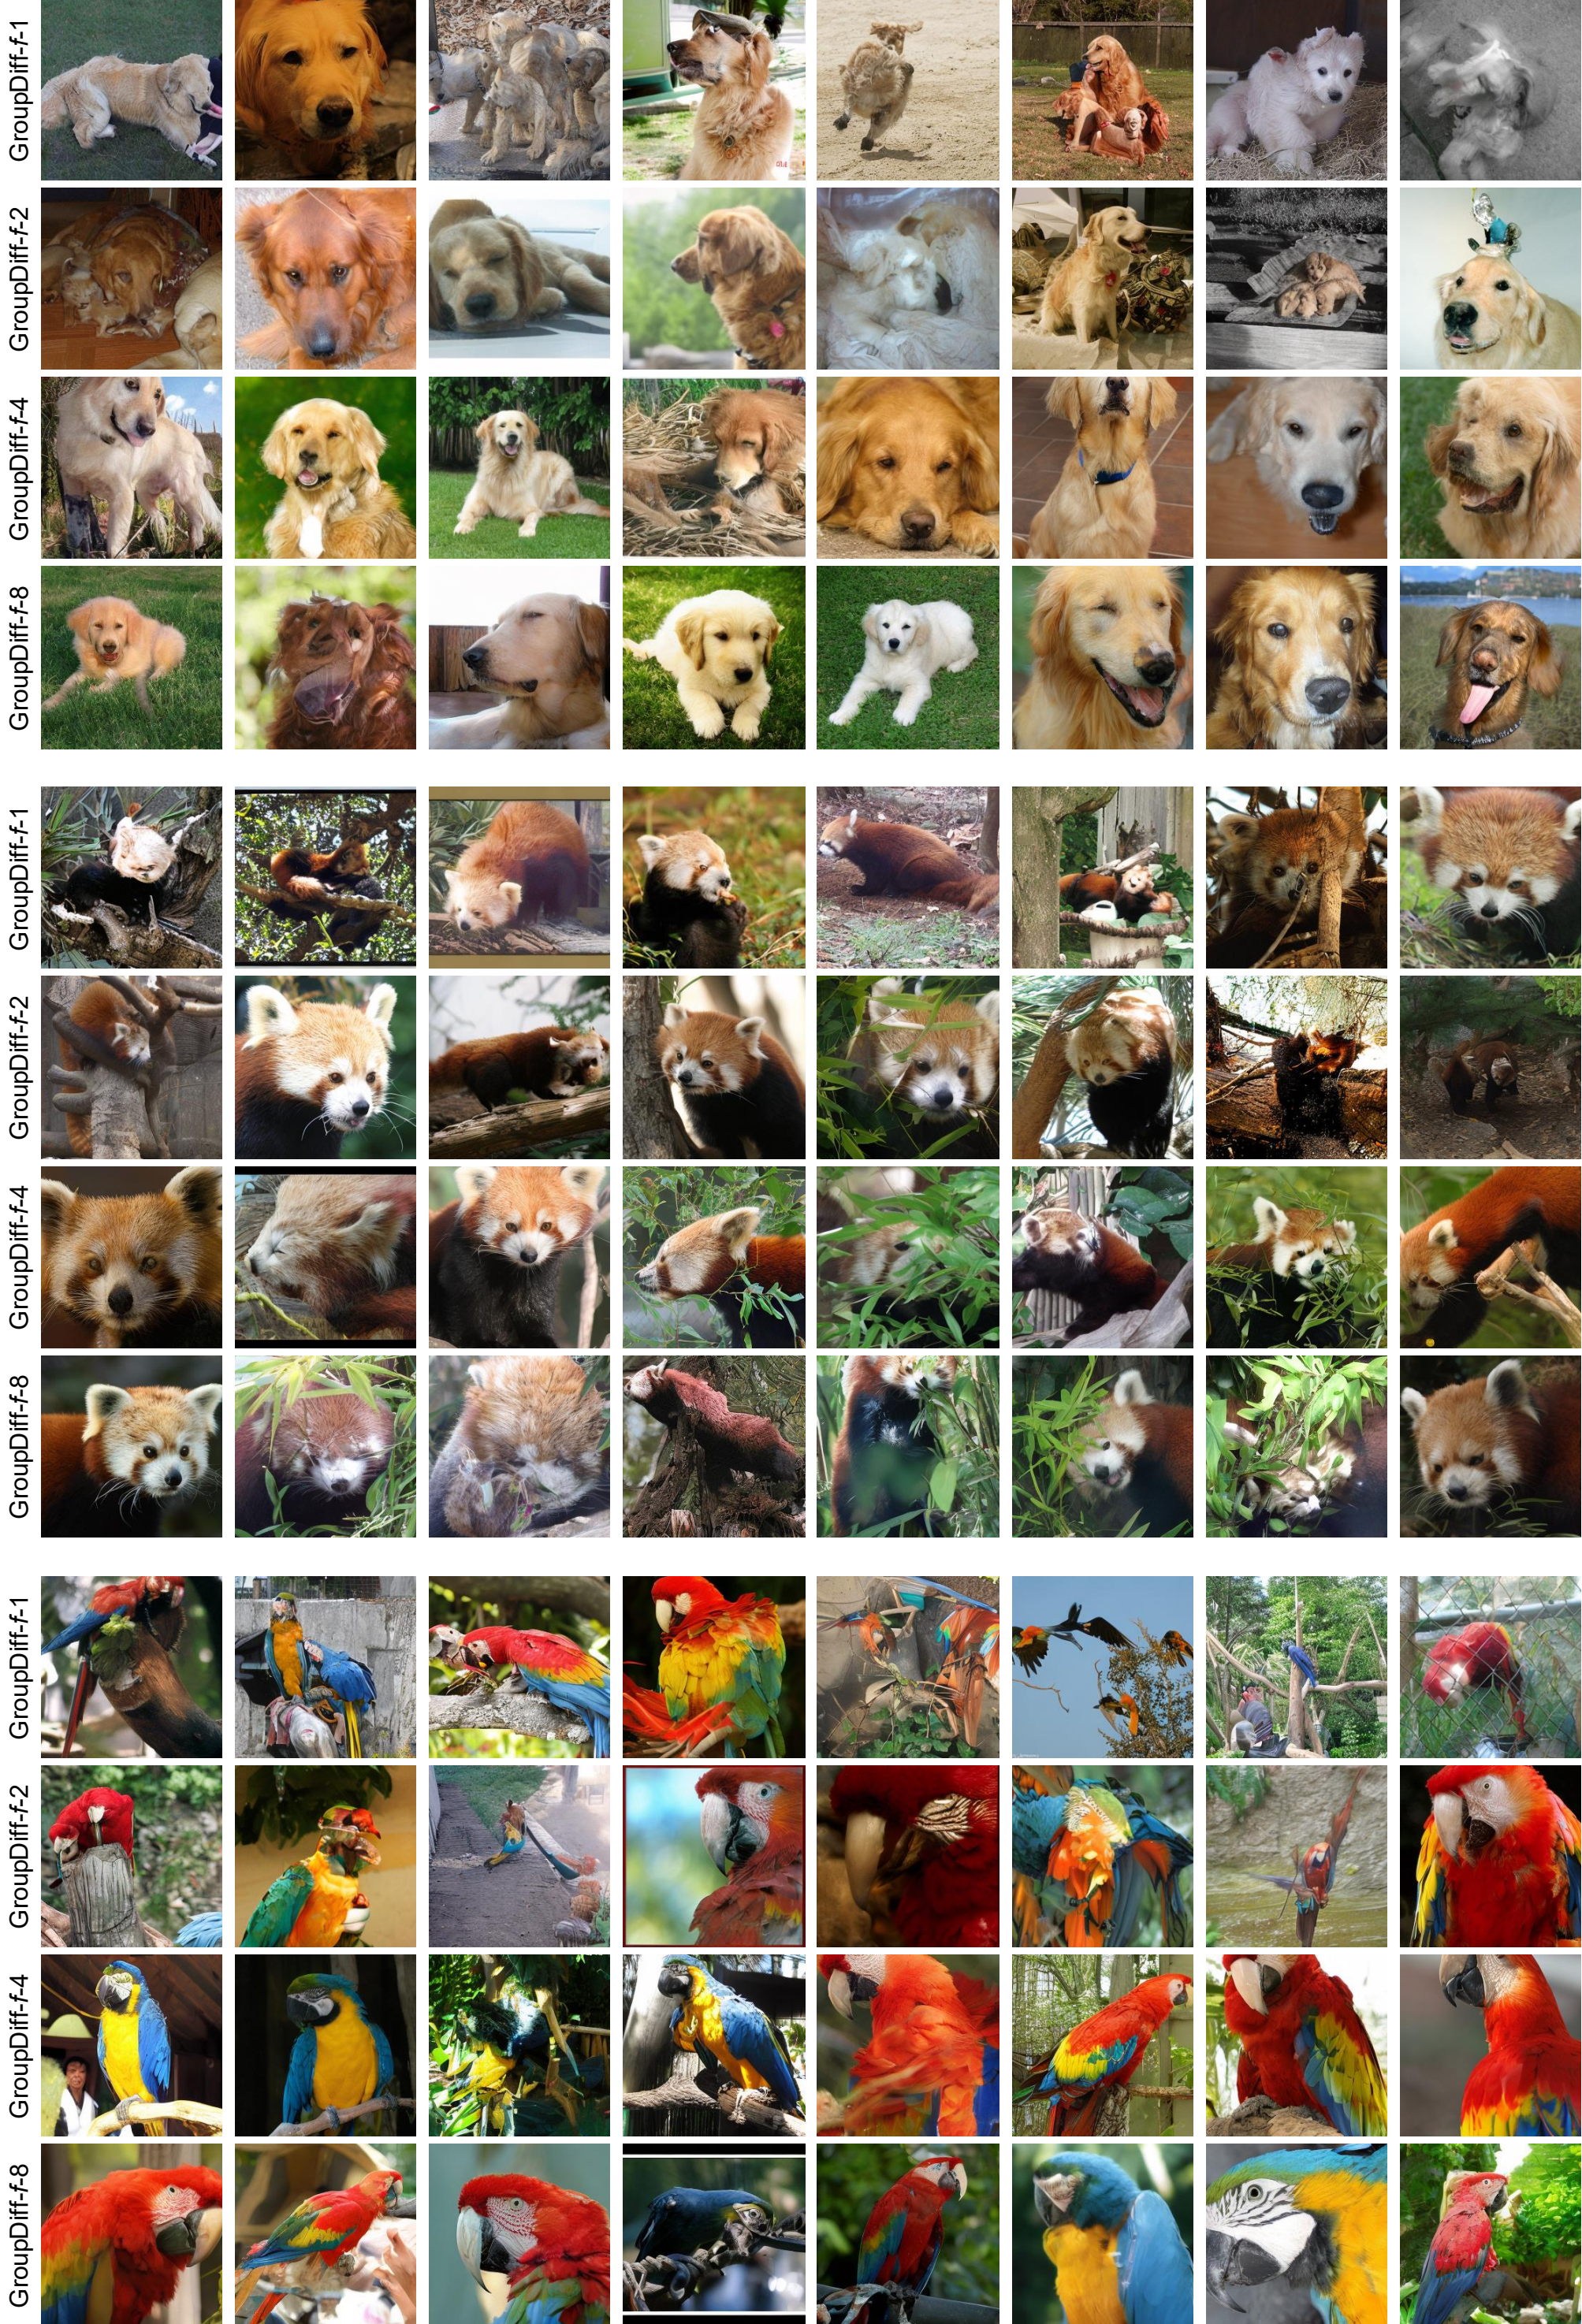



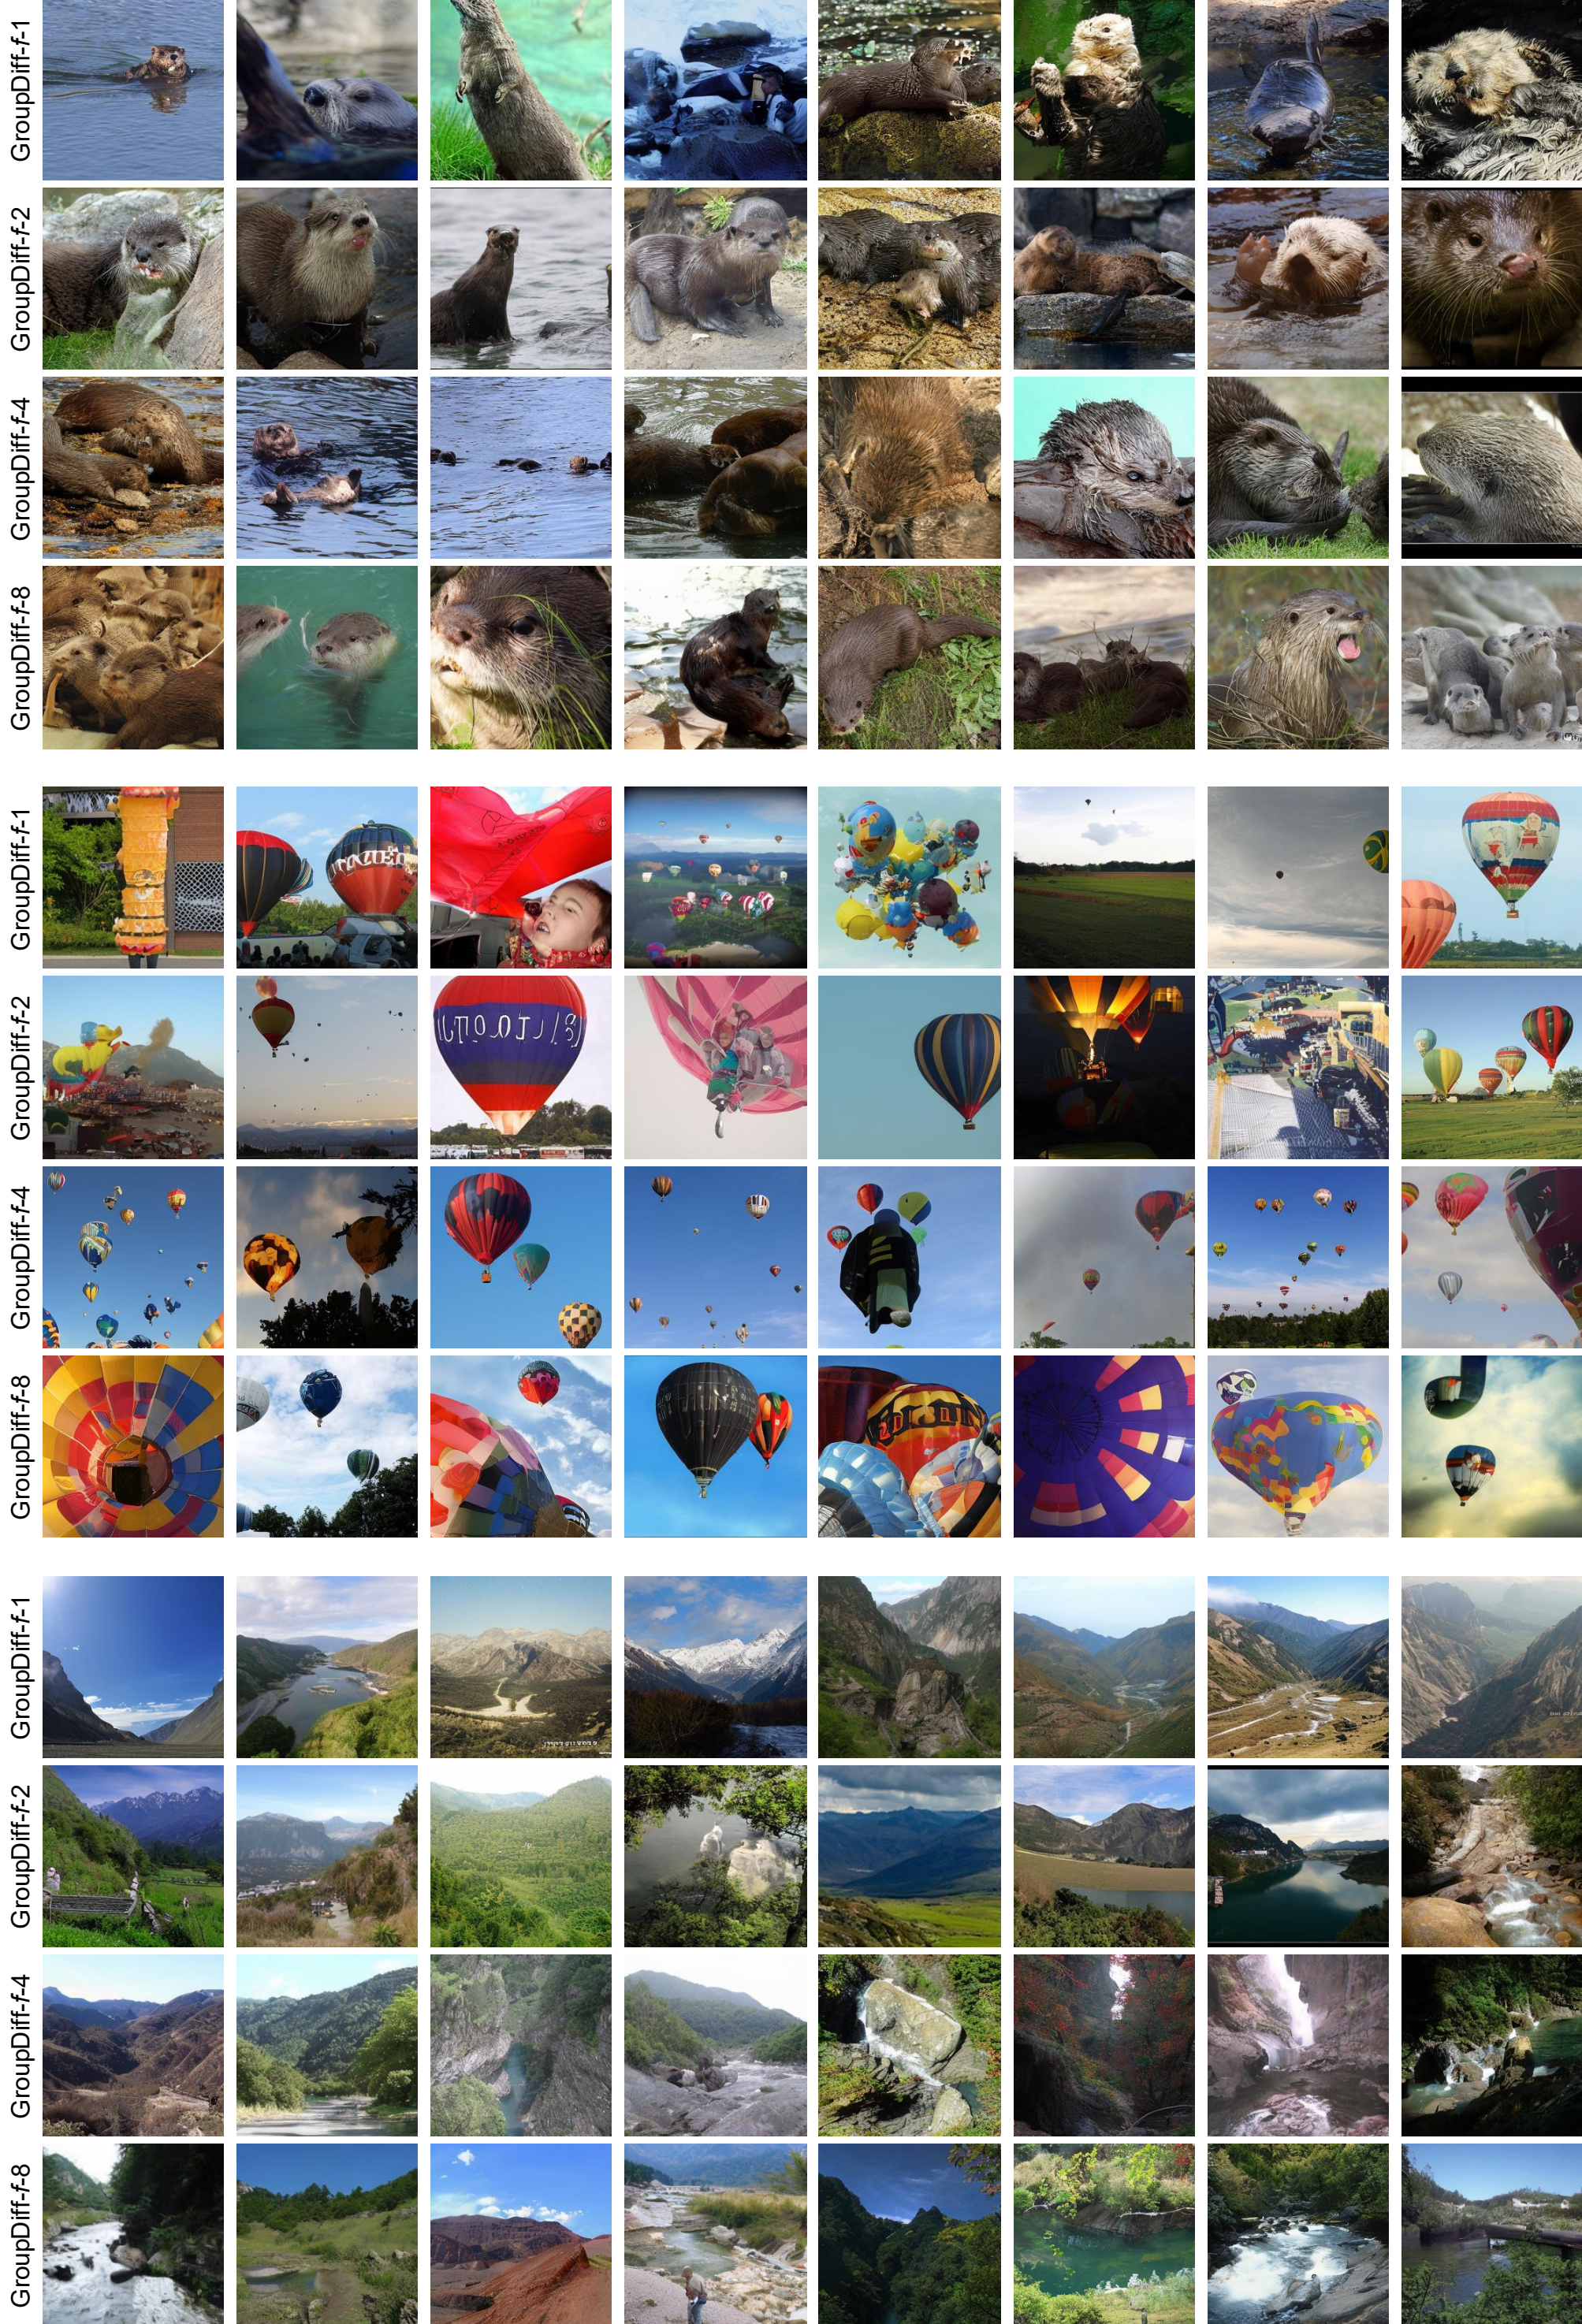

Supplement: Supplementary file 1 [file groupdiff-supp-abl.pdf]
